# Supplementary material for: Quantifying identifiability to choose and audit $\epsilon$ in differentially private deep learning
Source: arXiv:2103.02913 source file (2021-07-20)
Supplement: Supplementary file 1 [file appendix.tex]

%\section{Appendix}
%\label{sec:append}
\begin{comment}

\section{Tail Bound Arguments for Maximum Confidence}
\label{subsec:tail-bound-seq-composition}

In Section \ref{sec:dp}, \epsdlt-DP and the Gaussian mechanism were introduced. Since choosing $\sigma>\Delta f_2\sqrt{2ln(1.25/\delta)}/\eps$ leads to loose bounds, we focused on the tight bounds offered by the RDP definition in the body of our paper. We now more closely analyze the traditional definition of DP, including sequential composition, as defined in Theorem \ref{def:seqcomposition}.

The choice of $\sigma=\Delta f_2\sqrt{2ln(1.25/\delta)}/\eps$ is based on the tail bounds of the Gaussian mechanism, which specify the maximum magnitude of noise for which $\eps$-DP holds, $\frac{\eps\sigma^2}{\Delta f_2}-\frac{\Delta f_2}{2}$. In an alternate proof of Theorem \ref{thrm:multidim-gauss}, we use the tail bound, rather than RDP properties, to differentiate between cases when $\eps$-DP holds and when it does not hold:
\begin{proof}
	Independent of the dimensionality $k$ we limit our notation to $\sgm$~since $\Sigma=\sgm\cdot\mathbb{I}$ and add i.i.d.~noise $\sim\cali{N}(0,\sgm)$ to $f(\cali{D})$. 
	Dwork et al.~\cite[p.~262]{dwork2014} showed that the tail bound $t$ bounds the the magnitude of the noise vector $\vec{n}$ added by the mechanism when $\eps$-DP holds: $\|\vec{n}\| \le t = \frac{\eps\sgm^2}{\Delta f_2}-\frac{\Delta f_2}{2}$.
	\begin{align}
	\beta(\cali{D}) &= \frac{\Pr(\cali{M}(\cali{D})=\vec{r})}{\Pr(\cali{M}(\cali{D})=\vec{r}) + \Pr(\cali{M}(\cali{D'})=\vec{r})} \nonumber \\
	& = \frac{1}{1 + \Pr(\cali{M}(\cali{D'})=\mathbf{r})/\Pr(\cali{M}(\cali{D})=\vec{r})} \label{eq:belief-multidim-general}\\
	& = \frac{1}{1 + e^{\left((\|\vec{r}-f(\cali{D})\|^2-\|\vec{r}-f(\cali{D'})\|^2)/2\sgm^2\right)}} \label{eq:belief_multidim_exact}
	\end{align}
	
	
	Note that $f(\cali{D})$ is maximally distinguishable from $f(\cali{D'})$ when noise is sampled in the opposite direction of $f(\cali{D'})$. This direction is specified by the unit vector $\frac{f(\cali{D'})-f(\cali{\cali{D}})}{\cali{S}(f)}=\frac{f(\cali{D'})-f(\cali{\cali{D}})}{\Delta f_2}$. Thus, by defining the radius of the spherical Gaussian distribution centered at $f(\cali{D})$ to be $t$, the added noise that leads to the maximal confidence of $\cali{A}_\var{prob}$ is $\vec{n}=\frac{f(\cali{D'})-f(\cali{D})}{\Delta f_2}\cdot\left(\frac{\eps\sgm^2}{\Delta f_2}-\frac{\Delta f_2}{2}\right)$. We know $\| \vec{r} \| \le \|f(\cali{D})+\vec{n}\|$ and continue from Equation \eqref{eq:belief_multidim_exact}:
	
	\begin{align}
	& \le \frac{1}{1+ e^{\frac{1}{2\sgm^2}(||f(\cali{D})+\vec{n}-f(\cali{D})||^2-||f(\cali{D})+\vec{n}-f(\cali{D'})||^2)}} \label{eq:add_tail}\\
	& = \frac{1}{1+ e^{\frac{1}{2\sgm^2}(||\vec{n}||^2-(||\vec{n}||+||f(\cali{D})-f(\cali{D'})||)^2)}} \label{eq:separate_tail}\\
	& = \frac{1}{1+ e^{\frac{1}{2\sgm^2}(t^2-(t+\Delta f)^2)}}\nonumber\\
	& = \frac{1}{1+ e^{\frac{-2t\Delta f+\Delta f^2}{2\sgm^2}}}\nonumber\\
	& = \frac{1}{1+ e^{\frac{-2\Delta f\left(\frac{\eps\sgm^2}{\Delta f}-\frac{\Delta f}{2}\right)+\Delta f^2}{2\sgm^2}}}\nonumber\\
	& = \frac{1}{1 + e^{-\eps}} \label{eq:belief-multidim-simplified}
	\end{align}

	The step from Equation \eqref{eq:add_tail} to \eqref{eq:separate_tail} is possible because we know that $\vec{n}$ and $f(\cali{D})-f(\cali{D'})$ point in opposite directions. 
    	
\end{proof}
For further intuition, we examine the specific case in which $f(\cali{D})=\vec{0}$ and $f(\cali{D'})=\vec{1}$. We simplify from Equation \eqref{eq:belief_multidim_exact}:
%\subsection{Example for Multidimensional Gaussian Belief}
%\label{subsec:multidim_gaussian_belief_example}

%We let $ f(D)=\vec{0}, f(D')=\vec{1}$.
\begin{align}
	%\beta(\cali{D}) &= \frac{\Pr(\cali{M}(\cali{D})=\vec{r})}{\Pr(\cali{M}(\cali{D})=\vec{r}) + \Pr(\cali{M}(\cali{D'})=\vec{r})} \nonumber \\\
	%& = \frac{1}{1 + \Pr(\cali{M}(\cali{D'})=\mathbf{r})/\Pr(\cali{M}(\cali{D})=\vec{r})} \nonumber\\
	\beta(\cali{D}) & = \frac{1}{1 + e^{\left((\|\vec{r}\|^2-\|\vec{r}-\vec{1}\|^2)/2\sgm^2\right)}} \nonumber \\
	& = \frac{1}{1 + e^{\frac{1}{2\sgm^2}\left(kr_i^2-k(r_i-1)^2\right)}} \nonumber\\
	& = \frac{1}{1 + e^{\frac{k}{2\sgm^2}\left(2r_i-1\right)}} \label{eq:example_multidim_belief}
\end{align}
	
As visualized in Figure \ref{fig:proof bound analysis}, we define the radius of the spherical Gaussian distribution centered at $f(D)$ to be $t$. We analyze the case where $t$ is at a $45^\circ$ angle to the origin and can apply the Pythagoran theorem. Then $t^2 = \sum_i^k(r_i)^2 = kr_i^2$ and $t = \frac{1}{\sqrt(k)}r_i$. We set $r_i = t\sqrt{k}$ and continue from Equation \eqref{eq:example_multidim_belief}:

	
	\begin{align}
	& \le \frac{1}{1 + e^{\frac{k}{2\sgm^2}\left(\frac{2}{\sqrt{k}}\left(\frac{-\eps\sgm^2}{\Delta f_2}+\frac{\Delta f_2}{2}\right)-1\right)}} \nonumber\\
	& = \frac{1}{1 + e^{\frac{k}{2\sgm^2}\left(\frac{2}{\sqrt{k}}\left(\frac{-\eps\sgm^2}{\sqrt{k}}+\frac{\sqrt{k}}{2}\right)-1\right)}} \nonumber\\
	& = \frac{1}{1 + e^{\frac{1}{2\sgm^2}\left(-2\eps\sgm^2\right)}} \nonumber\\
	& = \frac{1}{1 + e^{-\eps}} \nonumber
	\end{align}

The alternate proof and intuitive example use an approach similar to the original proof: identifying a condition that holds when \eps-DP does and using this condition to bound $\beta(\cali{D})$ in $1-\delta$ cases. This section confirmed that such an analysis is possible without RDP. 

	\begin{figure}[h]
		\centering    
		\includegraphics[width=1\linewidth]{figures/tailbound_proof_intuition.pdf}    
		\caption{Tailbound argument intuition}
		\label{fig:proof bound analysis}      
	\end{figure}

	\section{Tail Bound Arguments for Adaptive Belief}
	\label{subsec:tail-seq-composition}
	We examine the implications of sequential composition for adaptive beliefs with regard to the tail bounds. We expect $\beta_k(\cali{D})\le\rho(\sum_{i=1}^{k}\eps_{i})$ in between the tail bounds of the multivariate Gaussian mechanism since with probability $1-\dlt$~$M_{Gau}$ provides $\eps$-DP~\cite[p.~264]{dwork2014}. We know that $\rho(\eps_1 + \eps_2) = \frac{1}{1+e^{-(\eps_1 + \eps_2)}}$ and $\rho(\eps_1) = \frac{1}{1+e^{-\eps_1}}$. We use Equation \eqref{eq:adaptive-gauss-basic} to analyze adaptive beliefs:

	
	\begin{align}
		\beta_k(\cali{D}) & = \frac{1}{1+\prod_{i=1}^{k} \frac{\Pr(\cali{M}_{i}(\cali{D'})=r_i)}{\Pr(\cali{M}_{i}(\cali{D})=r_i)}} \label{eq:tails-adaptive-belief-append}\\
		& \le \frac{1}{1+\prod_{i=1}^{k} e^{-\eps_{i}}} = \frac{1}{1+e^{-\sum_{i=1}^{k}\eps_{i}}} = \rho(\sum_{i=1}^{k}\eps_{i}) \label{eq:bound-tails-adaptive-belief}
		%& = \frac{\Pr(\cali{M}_{2}(\cali{D})=\mathbf{r})(\frac{1}{1+e^{-\eps_1}})}{\Pr(\cali{M}_{2}(\cali{D})=\mathbf{r})(\frac{1}{1+e^{-\eps_1}})+\Pr(\cali{M}_{2}(\cali{D'})=\mathbf{r})(1-\frac{1}{1+e^{-\eps_1}})}\\
		%& = \frac{\frac{1}{1+e^{-\eps_1}}}{\frac{1}{1+e^{-\eps_1}}+\frac{\Pr(\cali{M}_{2}(\cali{D'})=\mathbf{r})}{\Pr(\cali{M}_{2}(\cali{D})=\mathbf{r})}(1-\frac{1}{1+e^{-\eps_1}})}\\
		%& = \frac{\frac{1}{1+e^{-\eps_1}}}{\frac{1}{1+e^{-\eps_1}}+e^{\left(\frac{-\|\mathbf{r}+\mathbf{v}\|^2+\|\mathbf{r}\|^2}{2\sgm^2}\right)}(1-\frac{1}{1+e^{-\eps_1}})}\\	
		%&\le \frac{\frac{1}{1+e^{-\eps_1}}}{\frac{1}{1+e^{-\eps_1}} + e^{\frac{-2\lambda\Delta f - \Delta f^2}{2\sgm^2}}(\frac{1+e^{-\eps_1}-1}{1+e^{-\eps_1}})}\\
		%&= \frac{\frac{1}{1+e^{-\eps_1}}}{\frac{1}{1+e^{-\eps_1}} + e^{\frac{-2\Delta f \left(\frac{2\eps\sgm^2+\Delta f^2}{2\sgm^2}\right)- \Delta f^2}{2\sgm^2}}(\frac{1+e^{-\eps_1}-1}{1+e^{-\eps_1}})}\\
		%&= \frac{\frac{1}{1+e^{-\eps_1}}}{\frac{1}{1+e^{-\eps_1}} + e^{-\eps_2}(\frac{1+e^{-\eps_1}-1}{1+e^{-\eps_1}})}\\
	%	&\le \frac{\frac{1}{1+e^{-\eps_1}}}{\frac{1}{1+e^{-\eps_1}} + e^{\frac{-r^2+2r-1}{2\sgm^2}}(\frac{1+e^{-\eps_1}-1}{1+e^{-\eps_1}})}\\
	%	&\le \frac{\frac{1}{1+e^{-\eps_1}}}{\frac{1}{1+e^{-\eps_1}} + e^{\frac{-r^2+2r-1}{2\sgm^2}}(\frac{1+e^{-\eps_1}-1}{1+e^{-\eps_1}})}\\
	%	&\le \frac{\frac{1}{1+e^{-\eps_1}}}{\frac{1}{1+e^{-\eps_1}} + e^{-\eps_2}(\frac{1+e^{-\eps_1}-1}{1+e^{-\eps_1}})}\\
		%& = \frac{1}{1+e^{-\eps_2}e^{-\eps_1}} = \rho(\eps_1 + \eps_2) \qed
	\end{align}
	
	In the step from Equation \eqref{eq:tails-adaptive-belief-append} to \eqref{eq:bound-tails-adaptive-belief}, we use simplifications already introduced in Equations \eqref{eq:belief-multidim-general} to \eqref{eq:belief-multidim-simplified}, which use the tail bound argument introduced at the beginning of this section.

%\subsection{Example for Adaptive Gaussian Belief}
%\label{subsec:adaptive-gaussian-belief-example}
	Another way to analyze composition is to treat composed Gaussian mechanism executions as a single, higher dimensional execution with an adjusted \epsdlt guarantee. We apply the helpful fact, that the multiplication of independent Gaussian distributions results in a multinomial joint distribution. We can transform:
	\begin{align*}
		\beta_k(\cali{D}) = \frac{1}{1+\frac{\prod_{i=1}^{k}\Pr(\cali{M}_{i}(\cali{D'})=r_i)}{\prod_{i=1}^{k}\Pr(\cali{M}_{i}(\cali{D})=r_i)}} = \frac{1}{1+\frac{\cali{N}(\vec{\mu} = f(\cali{D'}), \Sigma )}{\cali{N}(\vec{\mu} = f(\cali{D}), \Sigma)}}
	\end{align*}
	We consider the example for which $\cali{N}(\vec{\mu}, \Sigma)$ is the multivariate normal distribution with mean $\vec{\mu} = \vec{0}$ or $\vec{\mu} = \vec{1}$ containing $k$ ones (or zeros) and covariance matrix $\Sigma = \sgm_i^2\cdot\mathbb{I}$. We have the same $\sgm_i$ in all dimensions as we assume that the privacy budget \epsdlt~ is split equally s. t. $\eps_i = \eps_j$ and $\dlt_i = \dlt_j$ which, given our previous assumptions, leads to $\sgm_i = \sgm_j, \forall i, j \in \{1,\ldots,k\}$. To show that $\rho_c$ holds again for composition we use an approach with tail bounds in each dimension $\mid r_i\mid \le \eps_i\sgm_i^2/\Delta f_{2_i} - \Delta f_{2_i}/2$.
	
	\begin{align*}
		\beta_k(\cali{D}) &= \frac{1}{1+\frac{\cali{N}(\vec{1}, \sgm_i^2\cdot\mathbb{I} )}{\cali{N}(\vec{0}, \sgm_i^2\cdot\mathbb{I})}} = \frac{1}{1+\frac{e^{-\|\vec{r}-\vec{1}\|/2\sgm_i^2}}{e^{-\|\vec{r}-\vec{0}\|/2\sgm_i^2}}}\\
		& = \frac{1}{1+e^{\frac{1}{2\sgm_i^2}(\|\vec{r}\|^2-\|\vec{r}-\vec{1}\|^2)}}
		\le \frac{1}{1+e^{\frac{1}{2\sgm_i^2}(kr_i^2-k(r_i-1)^2)}}\\
		&= \frac{1}{1+e^{\frac{k}{2\sgm_i^2}(2r_i-1)}} = \frac{1}{1+e^{\frac{k}{2\sgm_i^2}(2(-\eps_i\sgm_i^2/\Delta f_{2_i} + \Delta f_{2_i}/2)-1)}}\\
		&= \frac{1}{1+e^{\frac{k}{2\sgm_i^2}(2(-\eps_i\sgm_i^2/1 + 1/2)-1)}} = \frac{1}{1+e^{\frac{k}{2\sgm_i^2}(-2\eps_i\sgm_i^2)}}\\
		&= \frac{1}{1+e^{-k\eps_i}} = \rho(k\eps_i)
	\end{align*}

%\subsection{Composition of Adaptive Beliefs for \epsdlt-DP}
%\label{subsec:epsdlt_composition}


\section{Sequential Composition for Success Rate}
\label{subsec:seq_comp_success_rate}

The $k$-fold composition of $\cali{M}_{Gau_i}$, each step guaranteeing $(\eps_i,\dlt_i)$-DP, is represented by a single execution of $\cali{M}_{Gau}$ with $k$-dimensional output guaranteeing $(k\eps_i, k\dlt_i)$-DP. For analyzing $\rho_s$ under sequential composition, we will consider this representation. We make the following assumptions: output of $f_i(\cdot)$ corresponding to $\cali{M}_i$ is normalized s.t.~$f_i(\cali{D})=0$ and $f_i(\cali{D'})=1$ and $\Delta f_{2_i}=1$. Then, Definition~\ref{def:expected-adversarial-success-rate} yields

\begin{align*}
	\rho_s(\eps_i, \dlt_i, k) &\le 1 - \Phi\left(-\frac{\|\vec{0} - \vec{1}\|_2}{2\sgm_i}\right) \\
	& = 1 - \Phi\left(-\frac{\sqrt{k}}{2  (\sqrt{2ln(1.25/\dlt_i)}/\eps_i)}\right)\\
	&= 1 - \Phi\left(-\frac{\sqrt{k}\eps_i}{2\sqrt{2ln(1.25/\dlt_i)}}\right)
\end{align*}

The result shows that the strategy of $\cali{A}_{adapt}$ does not fully use the linear composition properties of $\eps_i$ and $\dlt_i$. Instead, $\eps_i$ grows in $\cali{O}(\sqrt{k})$ and $\dlt_i$ does not grow at all. Thus, $\rho_s(\eps_i, \dlt_i, k)$ slowly decreases when splitting the initial \epsdlt~ budget by larger $k$. This behavior is caused by the adaptive influence of every output $r_i$ of mechanism $\cali{M}_{Gau_i}$ has on the overall decision of $\cali{A}_{adapt}$. Eventually, the success rate converges against random guessing (0.5) when $k$ becomes large.

So, is there no good strategy for adversaries to avoid declining success rates with sequentially composed queries? Apparently, the best strategy so far is to not split, i.e., using $k=1$ and using the whole privacy budget at once. Considering this as possible worst case, any data owner should anticipate this which is why the bound for $\rho_s(\eps, \dlt)$ given in Definition~\ref{def:expected-adversarial-success-rate} is valid guidance for the level of protection. Hence, we will refer to this when evaluating privacy levels and regimes.



%\begin{align*}
%	r&=-\frac{\eps\sgm^2}{\Delta f_2}+\frac{\Delta f_2}{2},\\
%	\beta_2(\cali{D}, \beta_1(\cali{D})) &=  \frac{\Pr(\cali{M}_{2}(\cali{D})=r)\beta_1(\cali{D})}{\Pr(\cali{M}_{2}(\cali{D})=r)\beta_1(\cali{D}) + \Pr(\cali{M}_{2}(\cali{D'})=r)(1-\beta_1(\cali{D}))}\\
%	& = \frac{\Pr(\cali{M}_{2}(\cali{D})=r)(\frac{1}{1+e^{-\eps_1}})}{\Pr(\cali{M}_{2}(\cali{D})=r)(\frac{1}{1+e^{-\eps_1}})+\Pr(\cali{M}_{2}(\cali{D'})=r)(1-\frac{1}{1+e^{-\eps_1}})}\\
%	& = \frac{\frac{1}{1+e^{-\eps_1}}}{\frac{1}{1+e^{-\eps_1}}+\frac{\Pr(\cali{M}_{2}(\cali{D'})=r)}{\Pr(\cali{M}_{2}(\cali{D})=r)}(1-\frac{1}{1+e^{-\eps_1}})}\\
%	& = \frac{\frac{1}{1+e^{-\eps_1}}}{\frac{1}{1+e^{-\eps_1}}+e^{\left(\frac{-\left(r-\Delta f_2\right)^2+r^2}{2\sgm^2}\right)}(1-\frac{1}{1+e^{-\eps_1}})}\\	
%	&\le \frac{\frac{1}{1+e^{-\eps_1}}}{\frac{1}{1+e^{-\eps_1}} + e^{\frac{2\left(\frac{\eps_2\sgm^2}{\Delta f_2}+\frac{\Delta f_2}{2}\right)-1}{2\sgm^2}}(\frac{1+e^{-\eps_1}-1}{1+e^{-\eps_1}})}\\
%	&= \frac{\frac{1}{1+e^{-\eps_1}}}{\frac{1}{1+e^{-\eps_1}} + e^{\frac{2\left(\eps_2\sgm^2+\frac{1}{2}\right)-1}{2\sgm^2}}(\frac{1+e^{-\eps_1}-1}{1+e^{-\eps_1}})}\\
%	&= \frac{\frac{1}{1+e^{-\eps_1}}}{\frac{1}{1+e^{-\eps_1}} + e^{\frac{-2\eps_2\sgm^2}{2\sgm^2}}(\frac{1+e^{-\eps_1}-1}{1+e^{-\eps_1}})}\\
%	&= \frac{\frac{1}{1+e^{-\eps_1}}}{\frac{1}{1+e^{-\eps_1}} + e^{-\eps_2}(\frac{1+e^{-\eps_1}-1}{1+e^{-\eps_1}})}\\
%%	&\le \frac{\frac{1}{1+e^{-\eps_1}}}{\frac{1}{1+e^{-\eps_1}} + e^{\frac{-r^2+2r-1}{2\sgm^2}}(\frac{1+e^{-\eps_1}-1}{1+e^{-\eps_1}})}\\
%%	&\le \frac{\frac{1}{1+e^{-\eps_1}}}{\frac{1}{1+e^{-\eps_1}} + e^{\frac{-r^2+2r-1}{2\sgm^2}}(\frac{1+e^{-\eps_1}-1}{1+e^{-\eps_1}})}\\
%%	&\le \frac{\frac{1}{1+e^{-\eps_1}}}{\frac{1}{1+e^{-\eps_1}} + e^{-\eps_2}(\frac{1+e^{-\eps_1}-1}{1+e^{-\eps_1}})}\\
%	& = \frac{1}{1+e^{-\eps_2}e^{-\eps_1}} = \rho(\eps_1 + \eps_2) \qed
%\end{align*}

\end{comment}
